# Supplementary material for: Gaussian processes for choosing laser parameters for driven, dissipative Rydberg aggregates
Source: arXiv:1806.10368 source file (2018-06-27)
Supplement: Supplementary file 1 [file Rydberg_Gaussian_13_SI.pdf]

# Supplementary Information: Gaussian processes for choosing laser parameters for driven, dissipative Rydberg aggregates

**C D B Bentley and A Eisfeld**

Max Planck Institute for the Physics of Complex Systems, Nöthnitzer Strasse 38, 01187 Dresden, Germany

E-mail: `cbentley@pks.mpg.de, eisfeld@pks.mpg.de`

In this Supplementary Information (SI), we provide:

1. Additional cross-sections for the dimer (full numerical scans and Gaussian process predictions) and for the quadromer (Gaussian process predictions).
2. Predicted cross-sections for the quadromer, with a different center compared to the main text (the center is now chosen to be the parameters that provided the best value of the cost).
3. A discussion of the choice of cost function, and the effect of transience in the state dynamics on the resulting cost values.
4. Details of the numerical routine used throughout the main text.
5. A brief comparison with alternate numerical routines.

Submitted to: *J. Phys. B: At. Mol. Opt. Phys.*

## 1. Cost landscape: additional 2D cross-sections

In the main text, we included four 2D cross-sections for any given predicted cost landscape. This choice was for convenient and clear display of the results. In contrast, the performance measures were calculated based on the six 2D cross-sections formed by varying the control parameters $(\Omega_p, \Omega_c, \Delta_p, \Delta_c)$ in every combination of pairs. Here we display the six 2D cross-sections used for these calculations, for completeness.

In figure 1, the cross-sections obtained by scanning the cost landscape for two system atoms (the dimer) are shown. Figure 2 shows the cross-sections of the predicted cost landscape for the dimer, and the associated standard deviation. Similarly, figure 3 shows the predicted cost and standard deviation cross-sections for the quadromer. As in the main text, all of these cross-sections are centered at the same point $x$: $(\Omega_p, \Omega_c, \Delta_p, \Delta_c) = (37.1, 40.1, -26.6, -74.7)$. In each figure, we have marked the parameters that were used to calculate thermalization dynamics in figures 3 and 8 in the main text.

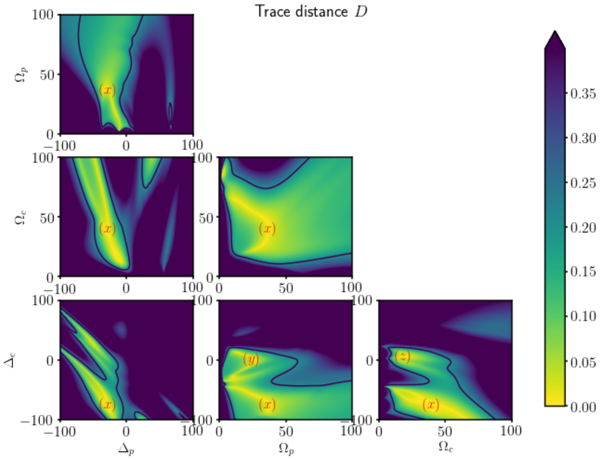


**Figure 1.** Six 2D cross-sections of the scanned cost landscape for the dimer (four were shown in figure 2 in the main text). The parameters marked by $(x)$, $(y)$ and $(z)$ are the parameters that generate the dynamics in the corresponding subplot of figure 3 in the main text. The center of the cross-sections is at $(x)$. The contour is at $D = 0.2$

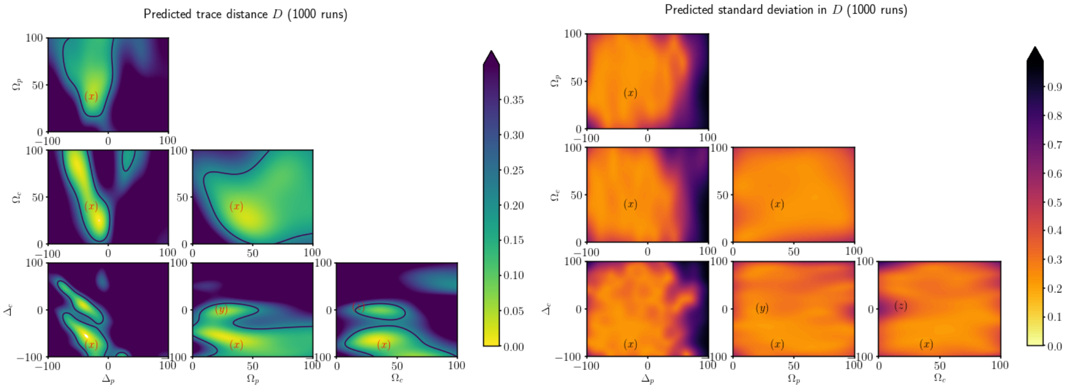


**Figure 2.** Predicted cost landscape (left) and standard deviation (right) for the dimer. The cross-sections were obtained after 1000 runs of a single instance of the numerical routine. As in figure 1, the parameters marked by $(x)$, $(y)$ and $(z)$ are the parameters that generate the dynamics in the corresponding subplot of figure 3 in the main text. The center of the cross-sections is at $(x)$.

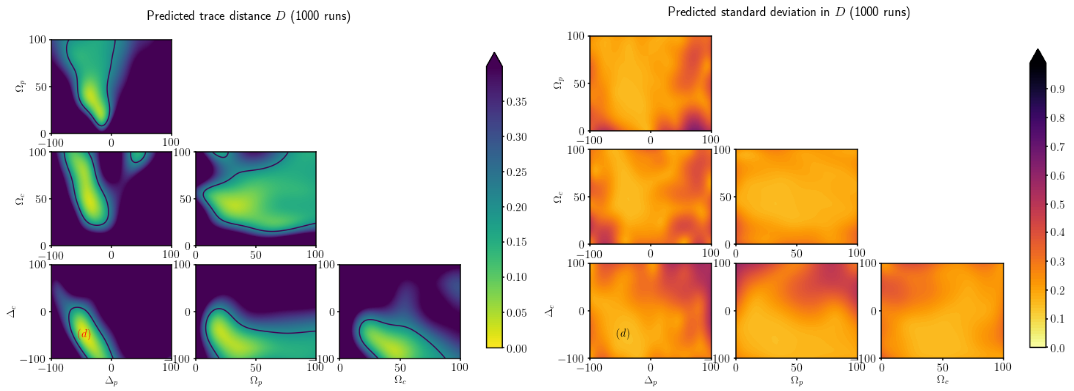


**Figure 3.** Predicted landscape (left) and standard deviation (right) for the quadromer, centered at the same point as for the dimer. The cross-sections were obtained after 1000 runs of the numerical routine. The parameters marked by $(d)$ are the parameters that generate the dynamics in the corresponding subplot of figure 8 in the main text.

## 2. Quadromer cross-sections: *best cost* center

In the main text (section 5), it was noted that the parameters providing the *best cost* for the quadromer were not those used as the center of the cross-sections for the dimer. Nonetheless, the cross-sections displayed for the quadromer (in section 5 of the main text and also in figure 3) were centered at $x$ (i.e. the same point as for the dimer), for comparison with the dimer cross-sections. In figure 4 we now include the cross-sections centered at the *best cost* parameters for the quadromer that were found by the numerical routine. This provides an additional snapshot of the predicted cost landscape, as well as displaying predicted lower-cost regions of the landscape.

In figure 4, one may observe similarities with the prediction performance for the cross-sections centered at $x$ in figure 3. The standard deviation in both cases is roughly 0.2, demonstrating consistency in the prediction of cost landscape over the full 4D parameter space. The performance measures (which depend on the given cross-sections) were calculated for the cross-sections in figure 4, and are displayed in figure 5. These are consistent with the performance measures displayed in figure 7 in the main text.

Note that there is nonzero standard deviation at the *best cost* point ($\sim$0.14). This is from the noise included in the regression model, which is discussed further in 4. Nevertheless, for the *best cost* parameters, the predicted and actual costs are very similar. This is also true for the other parameters evaluated to test their thermalization dynamics, which are marked in the cross-sections of figure 4. The predicted and actual costs are shown in figure 8 of the main text, which also shows the corresponding thermalization dynamics.

## 3. Non-steady trajectories with our cost choice ($D$)

In section 3 of the main text, we chose a final propagation time $t_f$, which fixed the time at which we compared the actual and target states. We are interested in states that thermalize, and $t_f$ fixes the maximal thermalization timescale. However, at time $t_f$ the propagated state may still be changing in time; it may not yet be steady.

In figure 6, we show the cost landscape comparison for $t_f = 2$ $\mu$s, as in the main text, and the steady state limit $t_f \to \infty$. Here the cross-sections are obtained by parameter scans for the dimer setup. Notice two effects in the cross-sections. First, new or extended low-cost regions appear in the steady state limit. This matches our expectation that larger permitted thermalization timescales allow more sets of parameters to generate the target thermal state. Second, there are also some regions where the cost increases. This occurs due to states that are transiently closer to the target state at the finite time $t_f = 2$ $\mu$s, then they approach a steady state with higher cost.

The first effect, where fixing a finite time $t_f$ limits the permitted thermalization timescale, is discussed in the main text (section 2.1).

In our case, the second (transient state) effect has little impact on the predicted cost landscapes. This

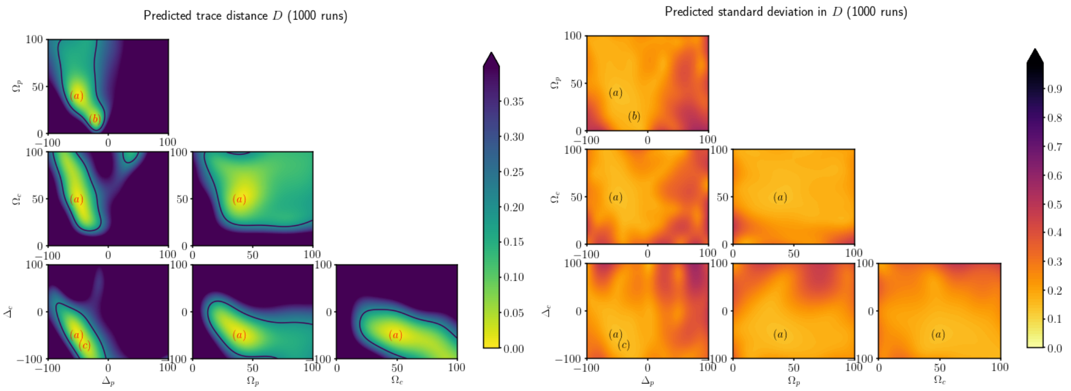


**Figure 4.** Predicted landscape (left) and standard deviation (right) centered at the best cost for the quadromer (marked by $(a)$). The cross-sections were obtained after 1000 runs of the numerical routine. The parameters marked by $(a) - (c)$ are the parameters that generate the dynamics in the corresponding subplot of figure 8 in the main text.

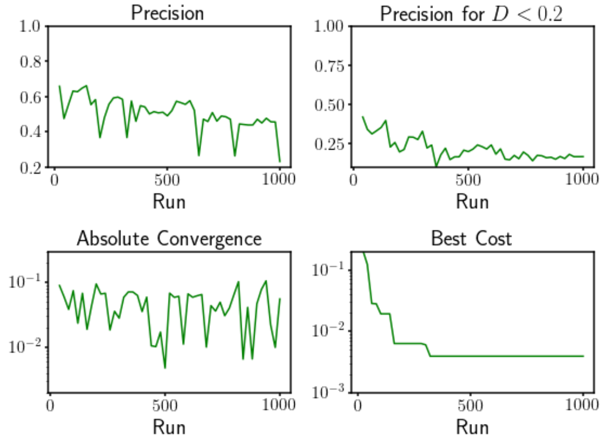


**Figure 5.** Intrinsic performance measures for the predicted landscape and standard deviation centered at the best cost for the quadromer, obtained from a single instance of the numerical routine.

effect is not particularly extensive (as seen in figure 6), and is also mainly in regions with high cost; we are less concerned with these regions. The changes in the cost $D$ due to non-steady, or transient, states are typically less than the predicted standard deviation in the cost. Additionally, for any parameters that are specifically evaluated, e.g. to examine their thermalization dynamics, it is straightforward to check that a steady state has been reached by the target time.

If the transience becomes significant, it is possible to choose a different cost function that minimizes this effect. For example, one could calculate the trace distance for each small time-step over an interval around $t_f$, and define the cost as the maximal trace distance obtained.

## 4. Numerical routine details

We have applied Gaussian processes to predict the cost landscape and its standard deviation for different physical setups. As discussed in the main text, we used previous predictions of the cost landscape to inform choices about the following parameters to evaluate. Using this active learning [1] approach, we obtained remarkably accurate predictions of the cost landscape using few simulations.

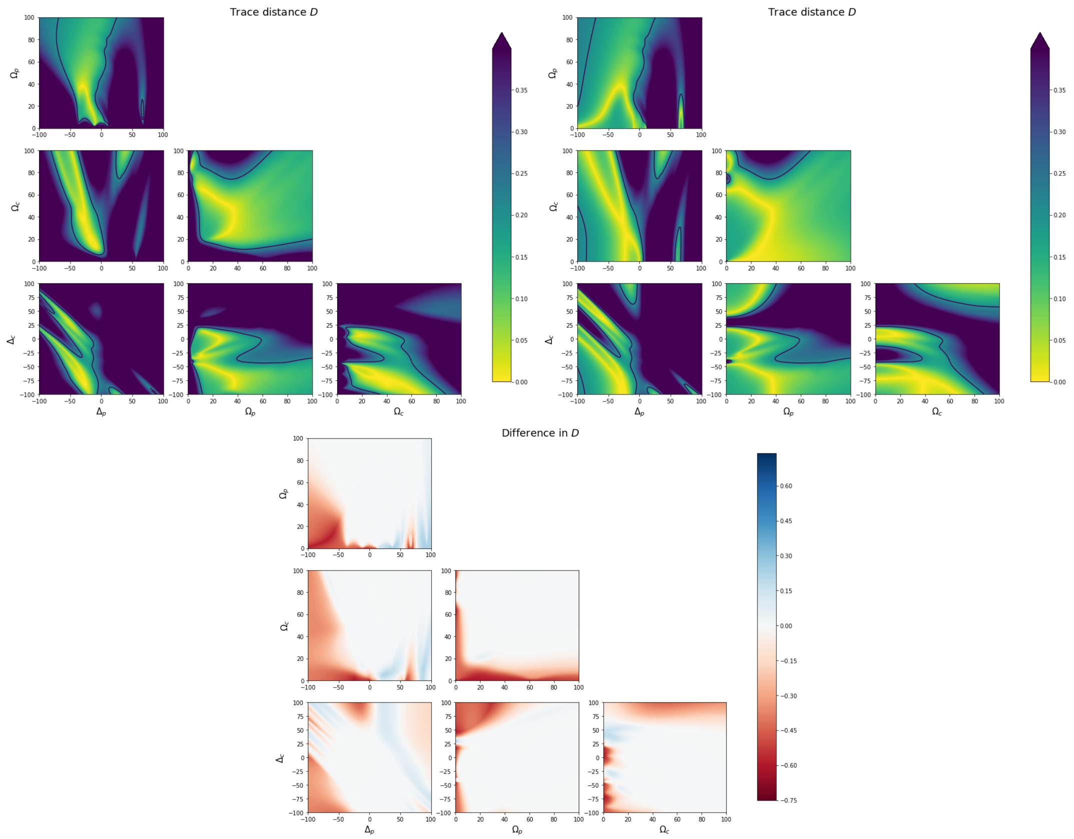


**Figure 6.** Cost landscape cross-sections for the dimer, obtained by parameter scans. The cost here is defined as the trace distance between the target thermal state and the actual state (top left) propagated for 2 $\mu$s, and (top right) calculated for the steady state. The bottom plot shows the difference between the top and middle landscape cross-sections. Each cross-section is centered at $x$.

### *4.1. Routine outline*

We used the Gaussian process optimizer in the M-LOOP package [2,3], which employs the Gaussian process regression algorithm (2.1) from [4] and implemented in scikitlearn [5]. The GP regression fits the cost function using known points in the cost landscape. This fit is then used to find the next parameters to evaluate, according to some selection criteria. There are various possible strategies to choose the next (test) point in the cost landscape. For example, points can be chosen to maximally reduce the standard deviation of the predicted cost landscape, or to explore the expected minimal region of the cost landscape, or a balance of these criteria. We used the default selection criteria in M-LOOP, which is a 'balanced' criteria dynamically sweeping between optimization and exploitation of the landscape: the parameters are selected using a (run-dependent) weighting of the predicted cost and the standard deviation of the predicted cost [3]. The specific parameters are found by searching the cost landscape (stochastically) for the minimal 'biased cost' that quantifies the selection criteria.

The numerical routine proceeds as follows:

(i) First, 11 initial 'training' runs are performed, with parameters chosen by differential evolution in our case. We refer to 'runs': a run involves choosing and evaluating a single set of parameters (a single point is obtained in the cost landscape).

(ii) Using the known points in the cost landscape, Gaussian process regression takes place to fit the cost landscape, and four sets of parameters are found based on the balanced selection strategy.

(iii) These parameters are evaluated, completing four runs (or less if fewer evaluations already mean that 1000 runs have been performed).

(iv) If 1000 runs have been performed, stop. If not, return to step 2.

The Gaussian process regression fits the known points in the cost landscape assuming a squared-exponential functional form for the covariance [6]. The regression includes optimizing 'hyper-parameters' that define lengthscales in the covariance function, as well as a noise term. It is possible to exclude the noise term, such that the GP will fit every observation exactly. We found, however, that including white noise improved the performance of the routine for our setup. Since the noise level is optimized as a hyper-parameter, we expect that it will decrease as more runs are performed.

The 1000-run stopping criteria is discussed in section 4.1 of the main text. The computational resources for the Gaussian process regression (using standard matrix inversion as in [6]) scale with the number of runs $n$ as $n^3$, and using the GP regression to predict the cost and its standard deviation for a given point scales as $n^2$ (p19 of [4]). For some $n$, we would thus require greater computational resources for the GP approach than for scanning the cost landscape. However, 1000 runs is well within the 'sweet spot' where it is computationally cheaper to use Gaussian processes for the dimer setup (note that the 'sweet spot' grows as each simulation becomes computationally more expensive).

Note that calculating the Gaussian process regression for the known points in the cost landscape, and then applying the parameter-selection strategy takes some time. During this calculation time, M-LOOP allows the option of using a standard optimization strategy to determine parameters to evaluate. We found that interspersing the Gaussian process optimization with a differential evolution [7] algorithm in this manner performed well; this is what we applied for the results in the manuscript. For slower Gaussian process regression or parameter-selection operations, more parameters are evaluated by differential evolution. In the following section, we compare the Gaussian process and differential evolution (GP+DE) case described here with alternate procedures.

## 5. Numerical routines: comparing parameter-selection procedures

Here we compare the performance measures, using different procedures to select parameters for evaluation. In the manuscript, we have applied the Gaussian process procedure interspersed with differential evolution (GP+DE). This interspersion is described above; the differential evolution algorithm selects parameters while the GP is calculating fits or parameters based on the predicted cost landscape. M-LOOP also allows one not to use differential evolution parameter selection during calculation for the GP-based procedure: we denote this case by GP. Alternately, the Gaussian process can be used to fit and predict the cost landscape after completion of all (1000) runs, using points solely determined by differential evolution: we denote this case by DE. The DE procedure is computationally slightly faster than the GP+DE procedure, while the GP procedure requires significantly more computational time.

The performance measures are shown in figure 7 for 100 instances of the different optimizer choices. The measures were calculated for each of the 100 instances, and the mean (solid line) and standard deviation (dashed) over instances are shown in the figure. This comparison is for the dimer, calculated as described in section 4.2 (and as performed for figure 5 for the GP+DE procedure) in the main text.

The GP procedure performs the worst of the three procedures in almost every performance measure in figure 7. A notable exception is the *best cost*, which is significantly better than the *best cost* from the GP+DE and DE procedures. For our physical setting, the GP procedure performs exceptionally well at finding the best cost, but not at predicting the cost landscape more generally.

The GP+DE and DE cases both perform very well. However, a couple of features of the active learning (GP+DE) approach made it preferable for our numerical routine. For the GP+DE procedure, there is continued improvement in the *accuracy* and both of the *precision* measures with the number of runs. The *accuracy* and *precision* measures also have significantly superior values after 1000 runs.

## References


[1] B. Settles, "Active Learning Literature Survey," Computer Sciences Technical Report 1648, University of Wisconsin–Madison, 2009.

[2] P. B. Wigley, P. J. Everitt, A. van den Hengel, J. W. Bastian, M. A. Sooriyabandara, G. D. McDonald, K. S. Hardman, C. D. Quinlivan, P. Manju, C. C. N. Kuhn, I. R. Petersen, A. N. Luiten, J. J. Hope, N. P. Robins, and M. R. Hush, "Fast machine-learning online optimization of ultra-cold-atom experiments," *Scientific Reports*, vol. 6, no. 25890, 2016.

[3] MLOOP source code and documentation found at URL: http://m-loop.readthedocs.io.

[4] C. E. Rasmussen and C. K. I. Williams, *Gaussian Processes for Machine Learning.* Cambridge: the MIT Press, 2006.

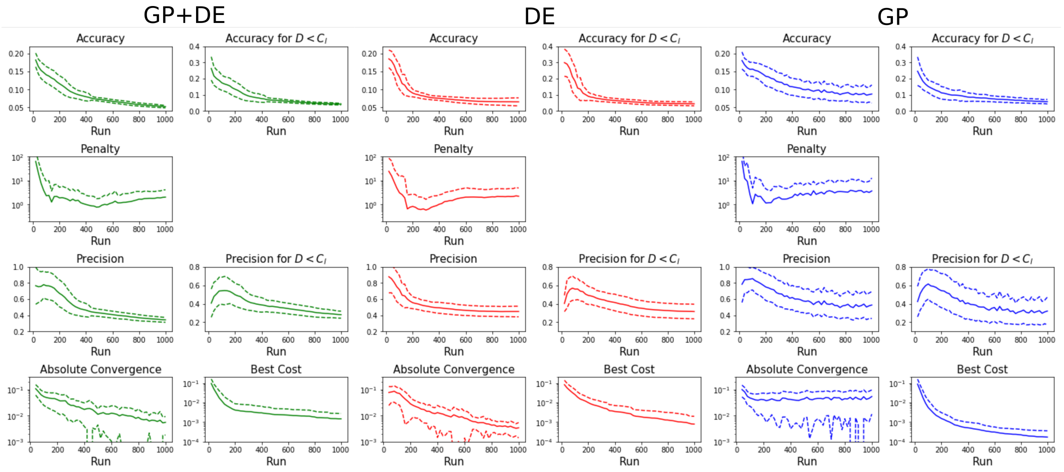


**Figure 7.** Performance measures for the dimer setup are shown for different numerical procedures. The procedures are denoted as follows. GP+DE: Gaussian process parameter selection interspersed with differential evolution. DE: differential evolution parameter selection. GP: Gaussian process parameter selection. The mean (solid) and standard deviation (dashed) over 100 instances of each procedure are shown. Where a standard deviation below the mean is consistently less than zero, this is not shown for clarity.

[5] F. Pedregosa, G. Varoquaux, A. Gramfort, V. Michel, B. Thirion, O. Grisel, M. Blondel, P. Prettenhofer, R. Weiss, V. Dubourg, J. Vanderplas, A. Passos, D. Cournapeau, M. Brucher, M. Perrot, and E. Duchesnay, "Scikit-learn: Machine Learning in Python," *J. Mach. Learn. Res.*, vol. 12, pp. 2825–2830, 2011.
[6] Scikit-learn documentation found at URL: http://scikit-learn.org/stable/modules/gaussian_process.html#gaussian-process.
[7] R. Storn and K. Price, "Differential Evolution - A Simple and Efficient Heuristic for Global Optimization over Continuous Spaces," *J. Global Optim.*, vol. 11, pp. 341–359, 1997.
